# Supplementary material for: ThinkGen: Generalized Thinking for Visual Generation
Source: arXiv:2512.23568 source file (2025-12-29)

*GenEval**WISEBench**ImgEdit**CVTG*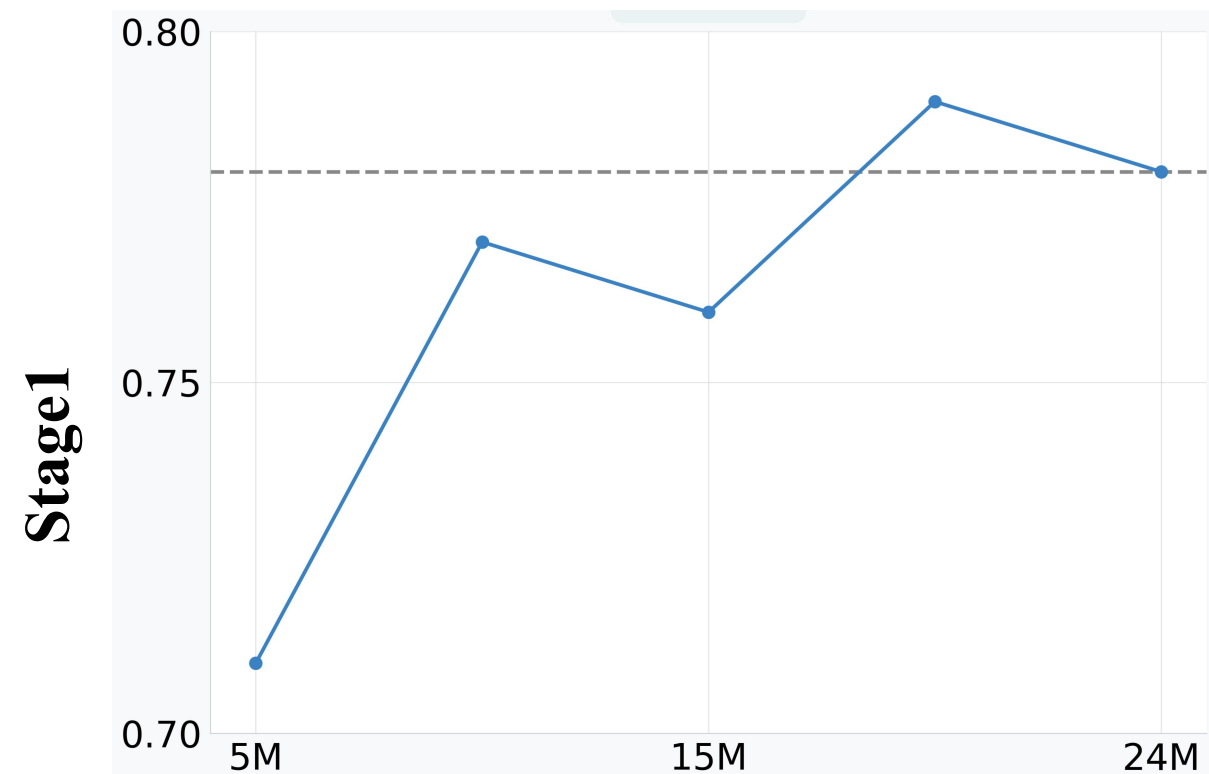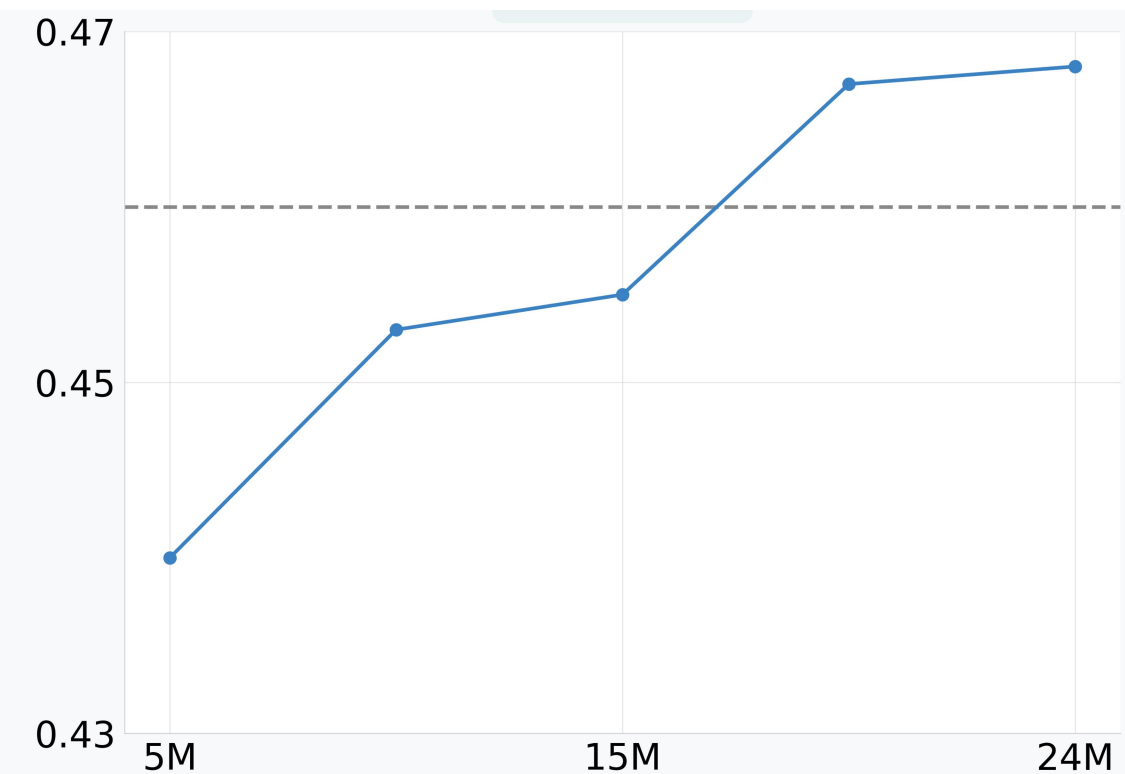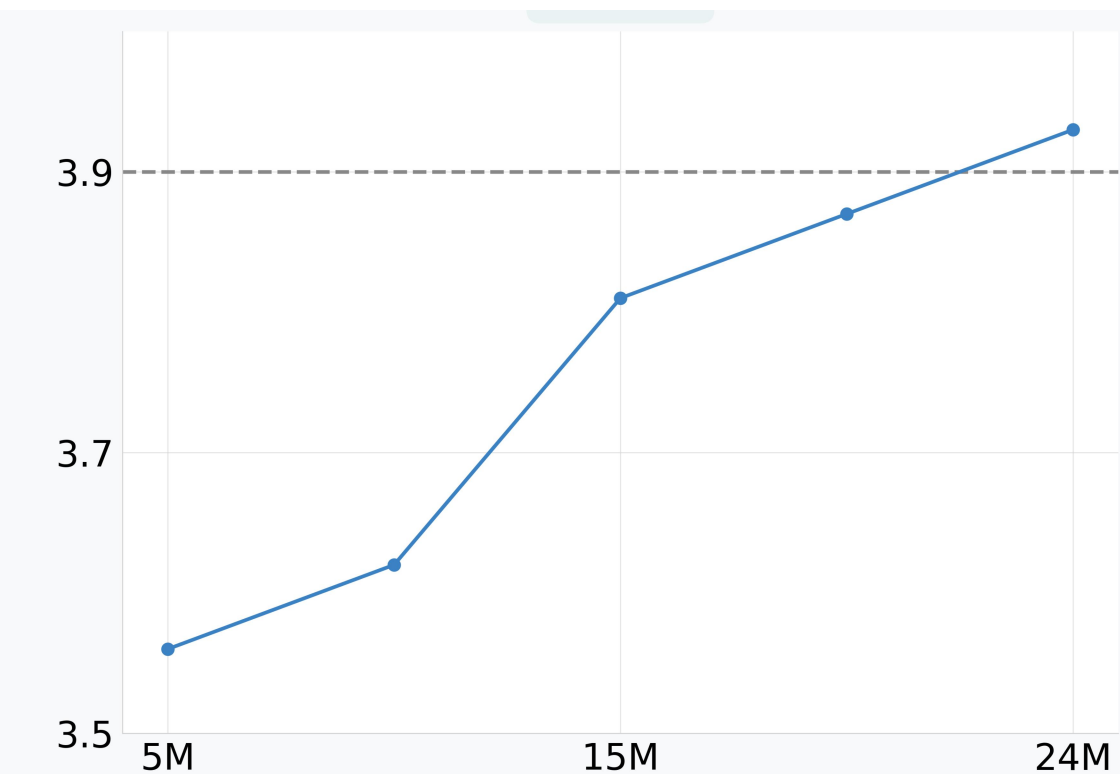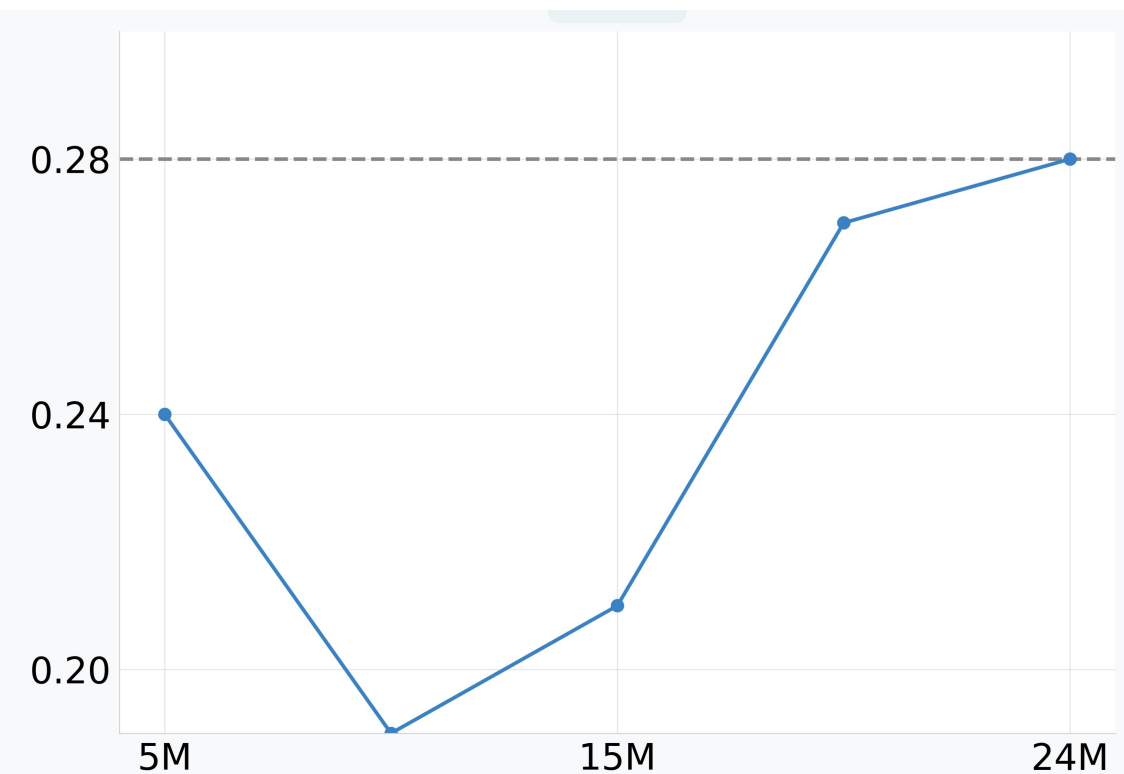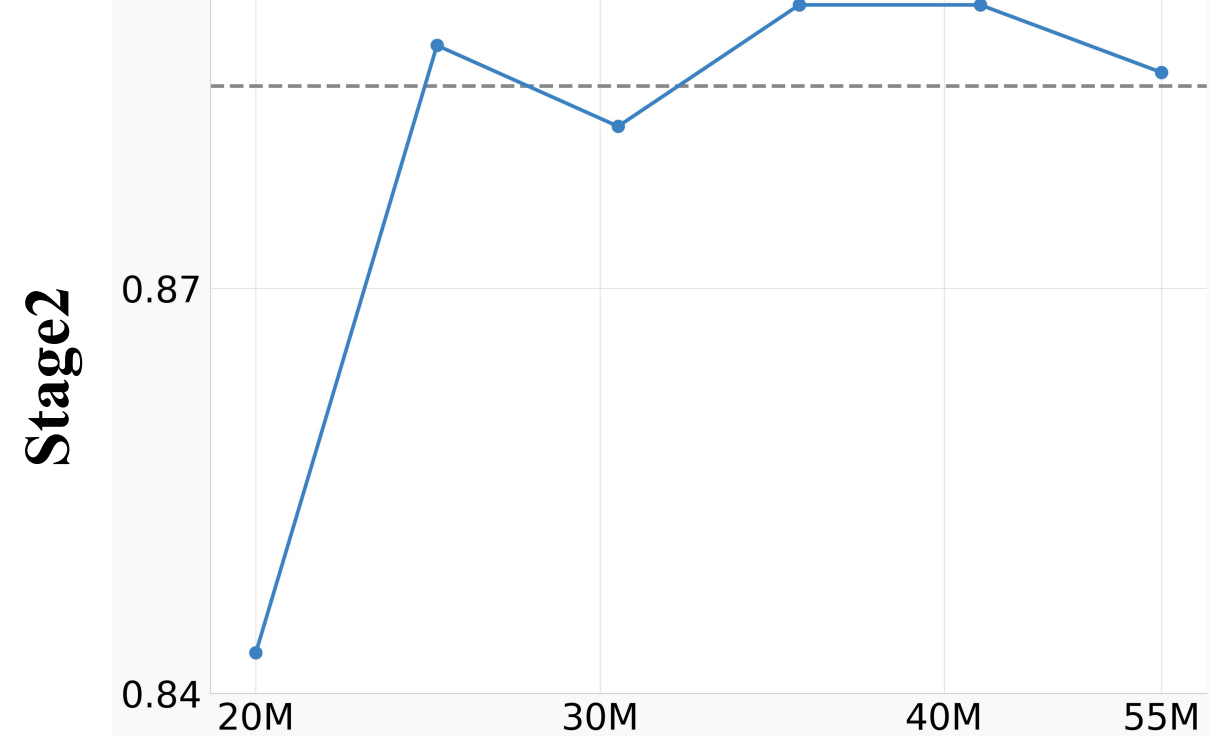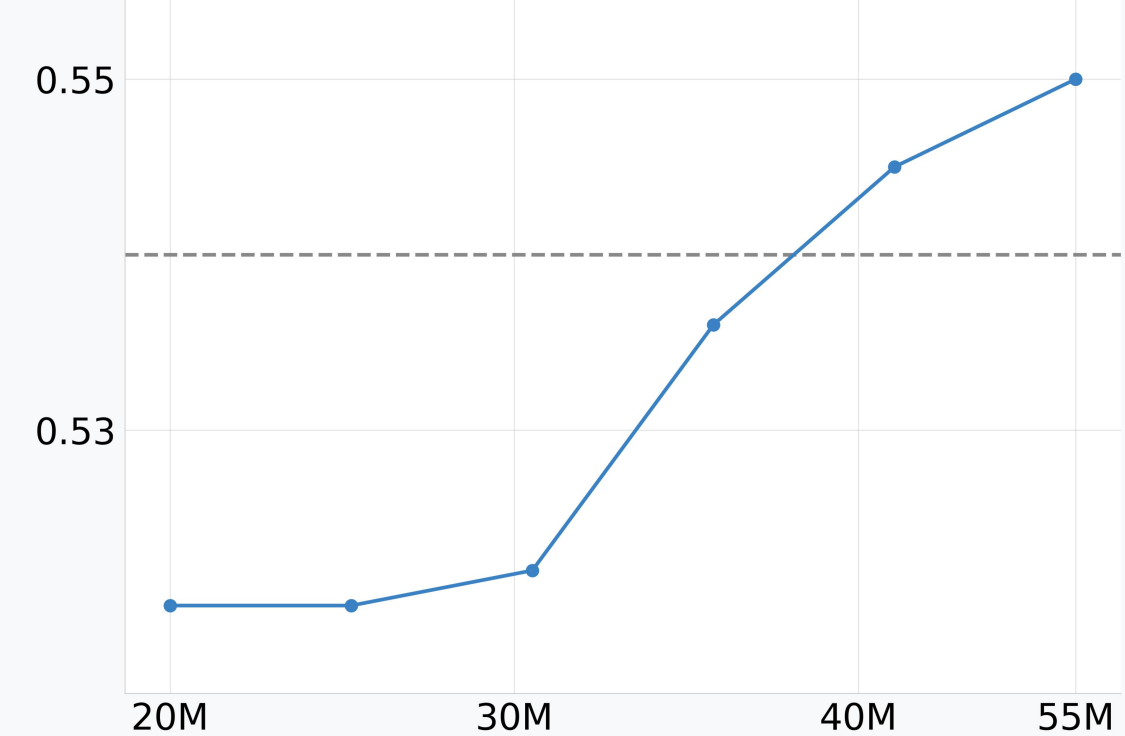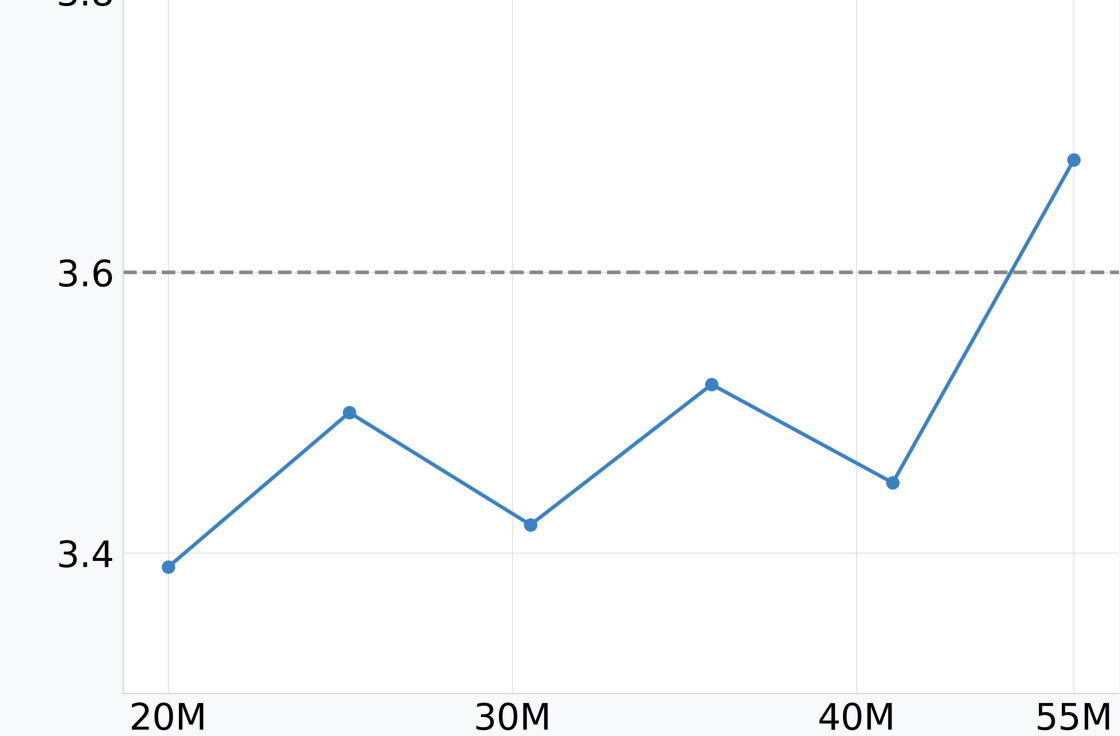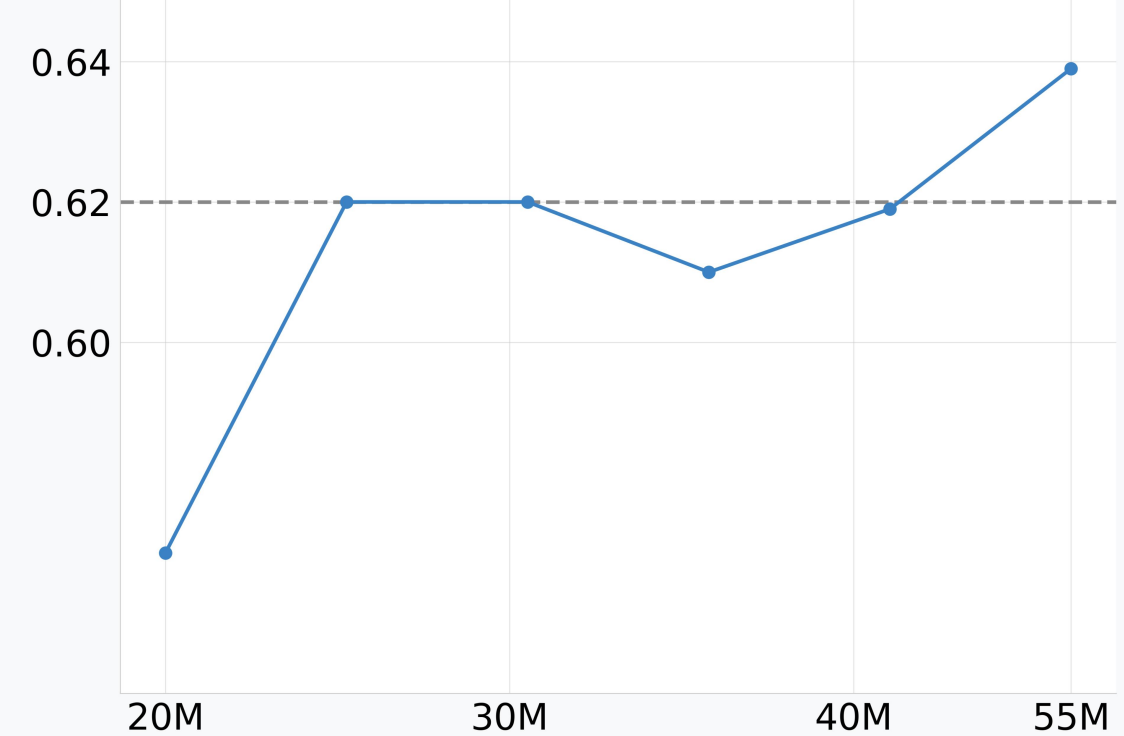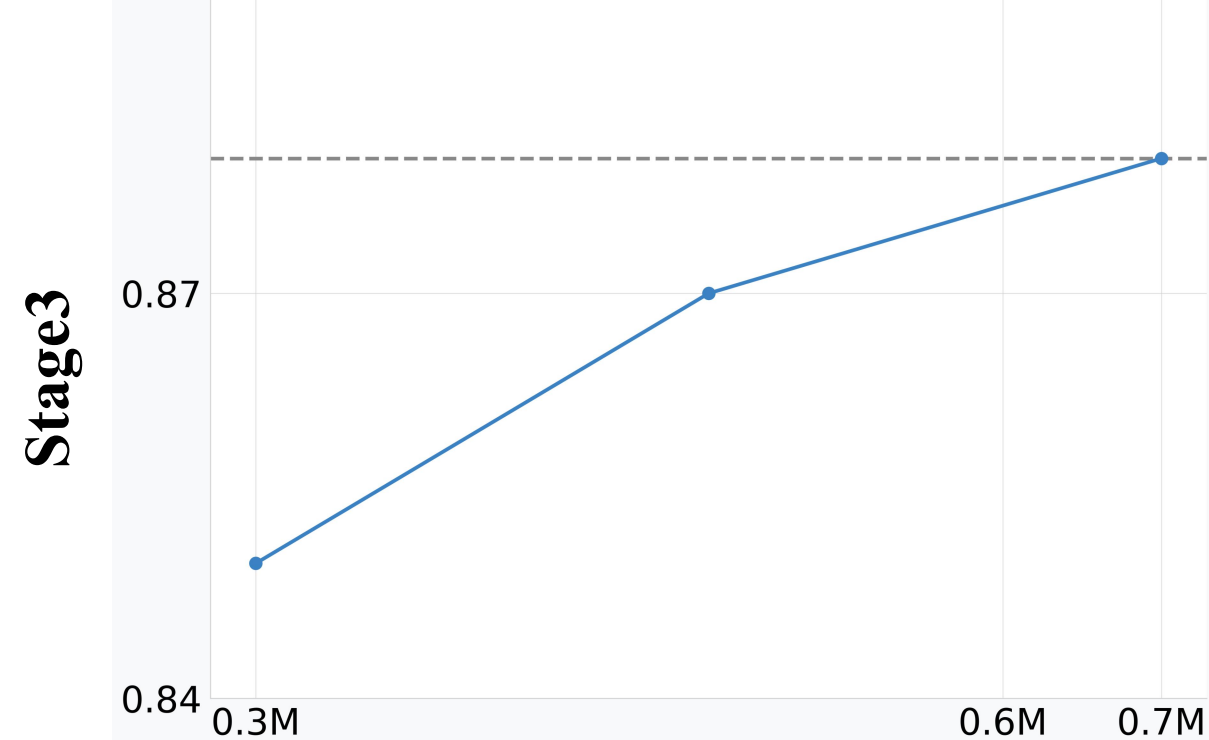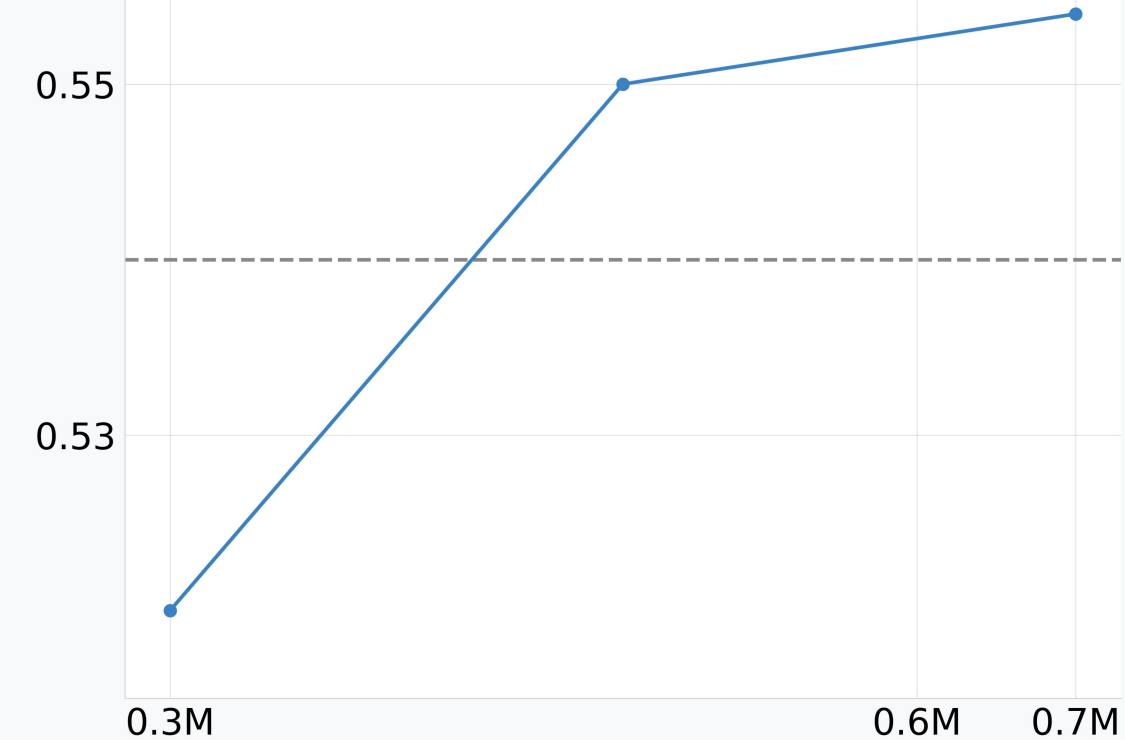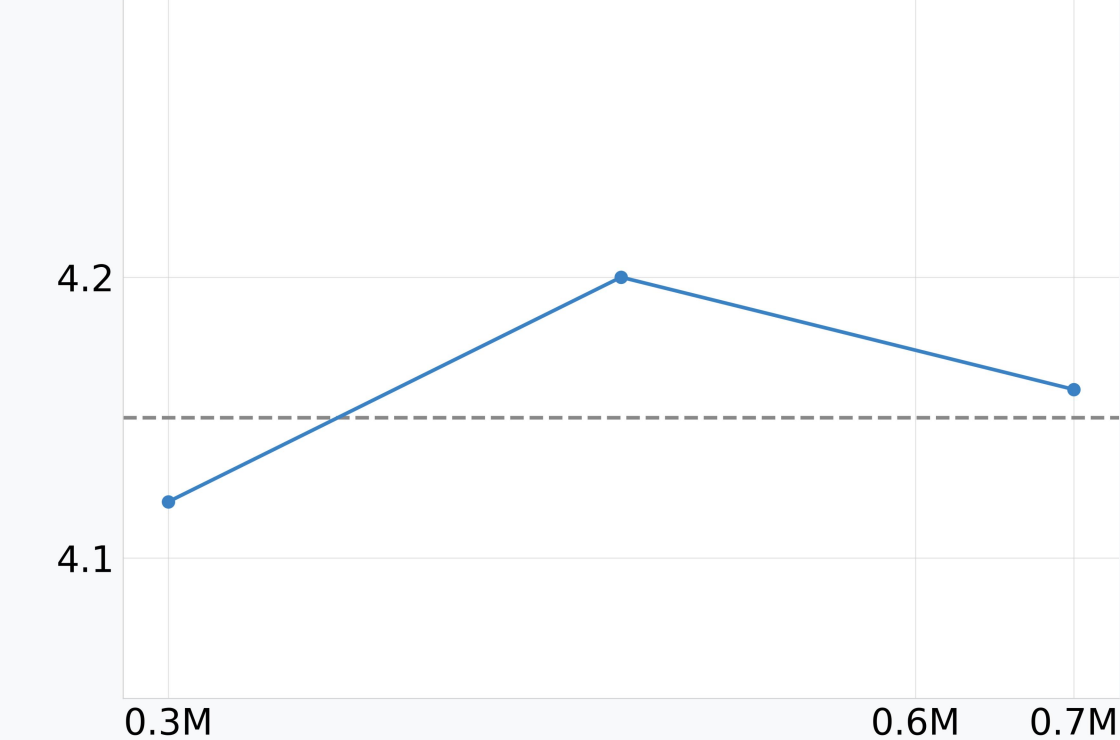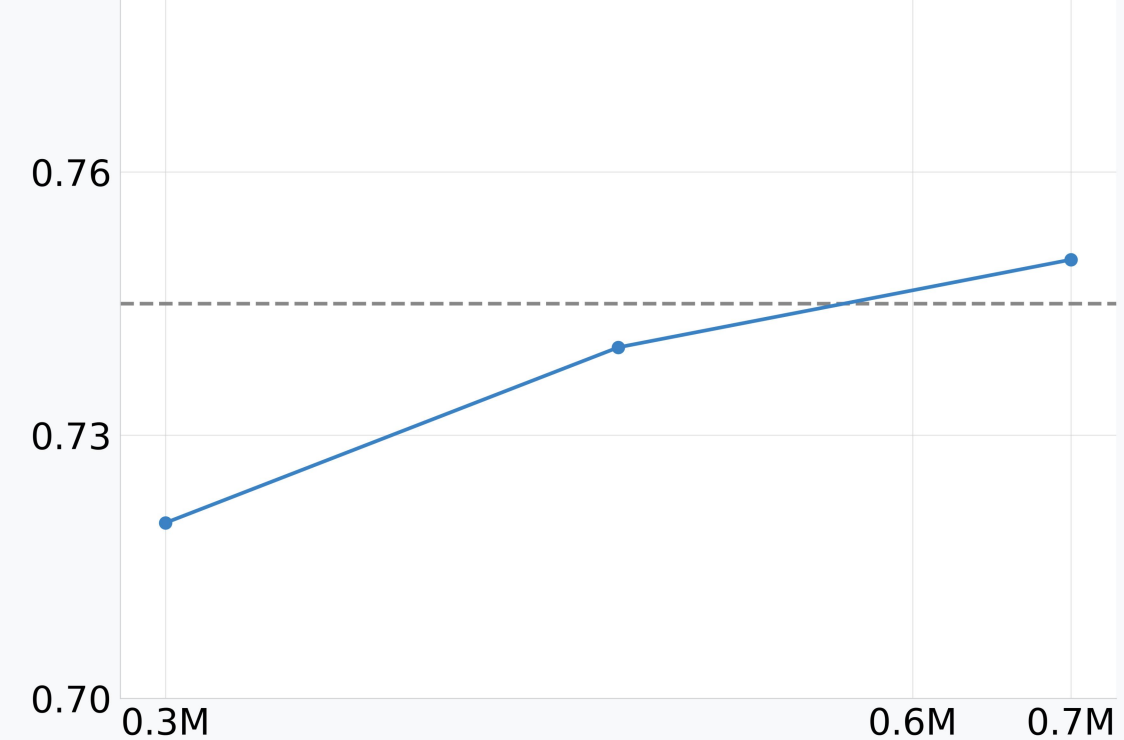

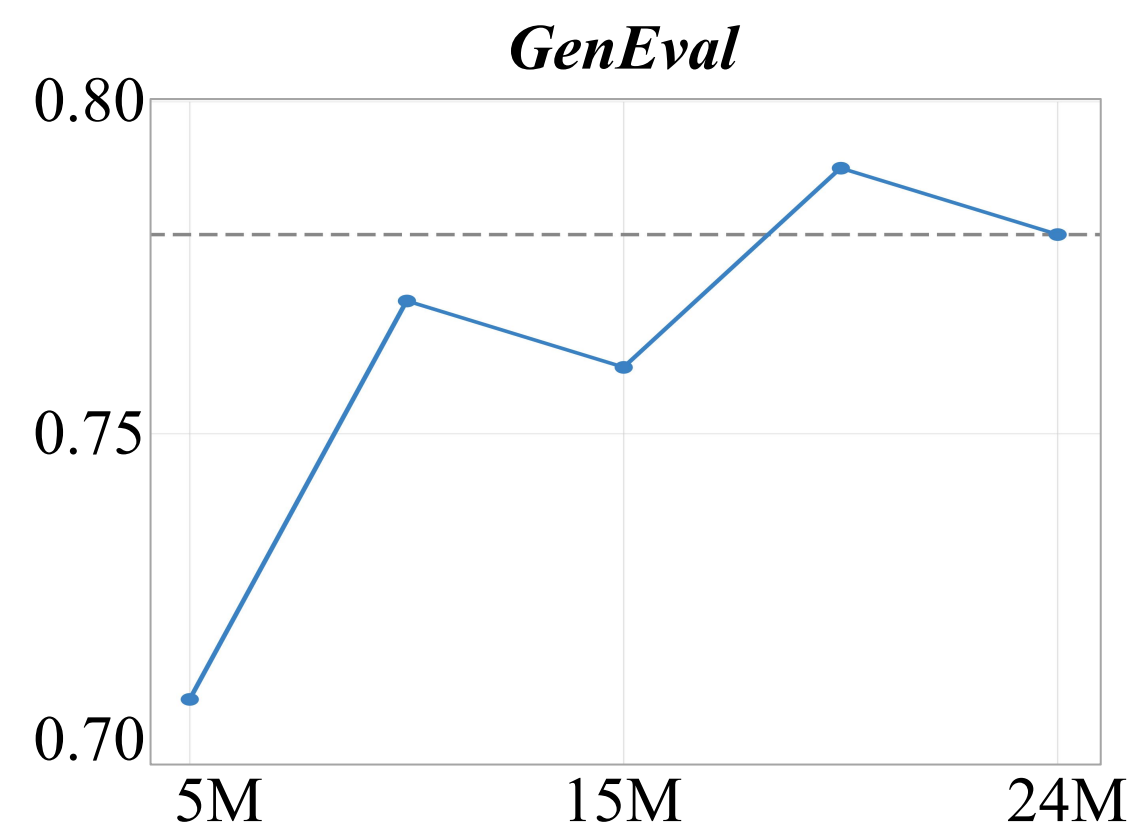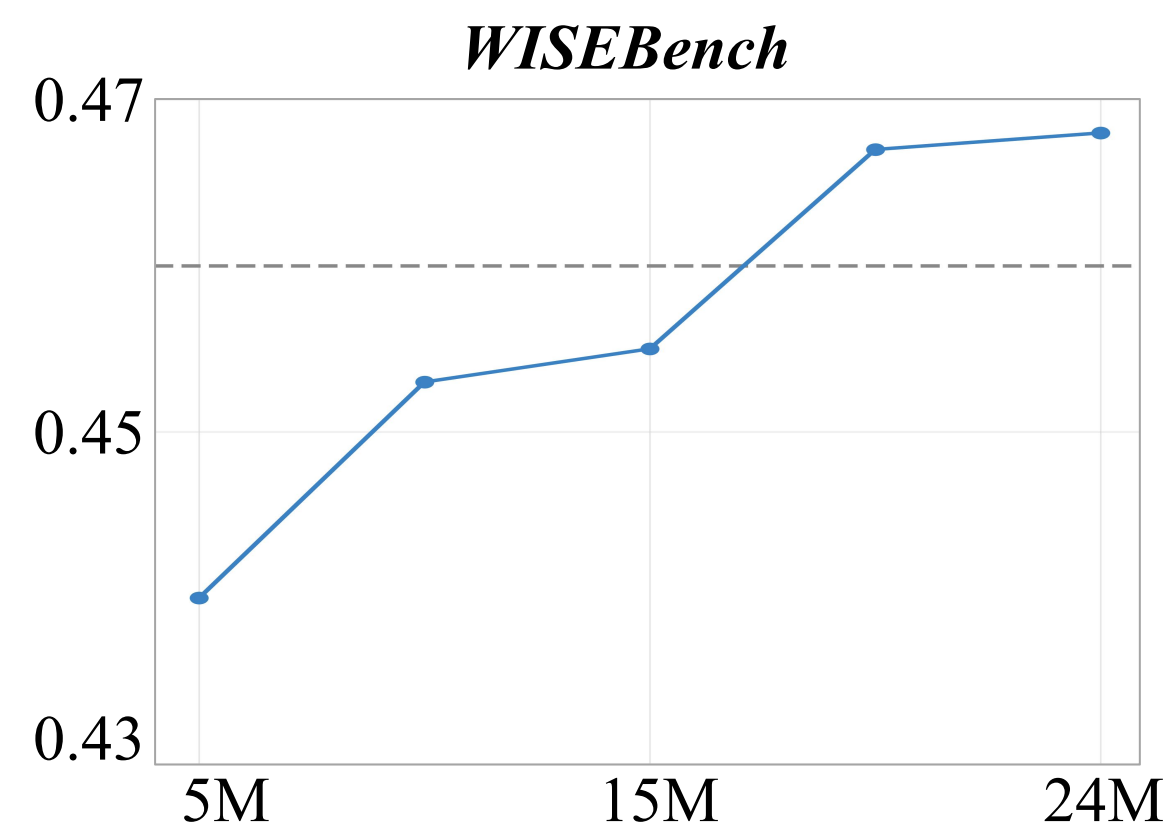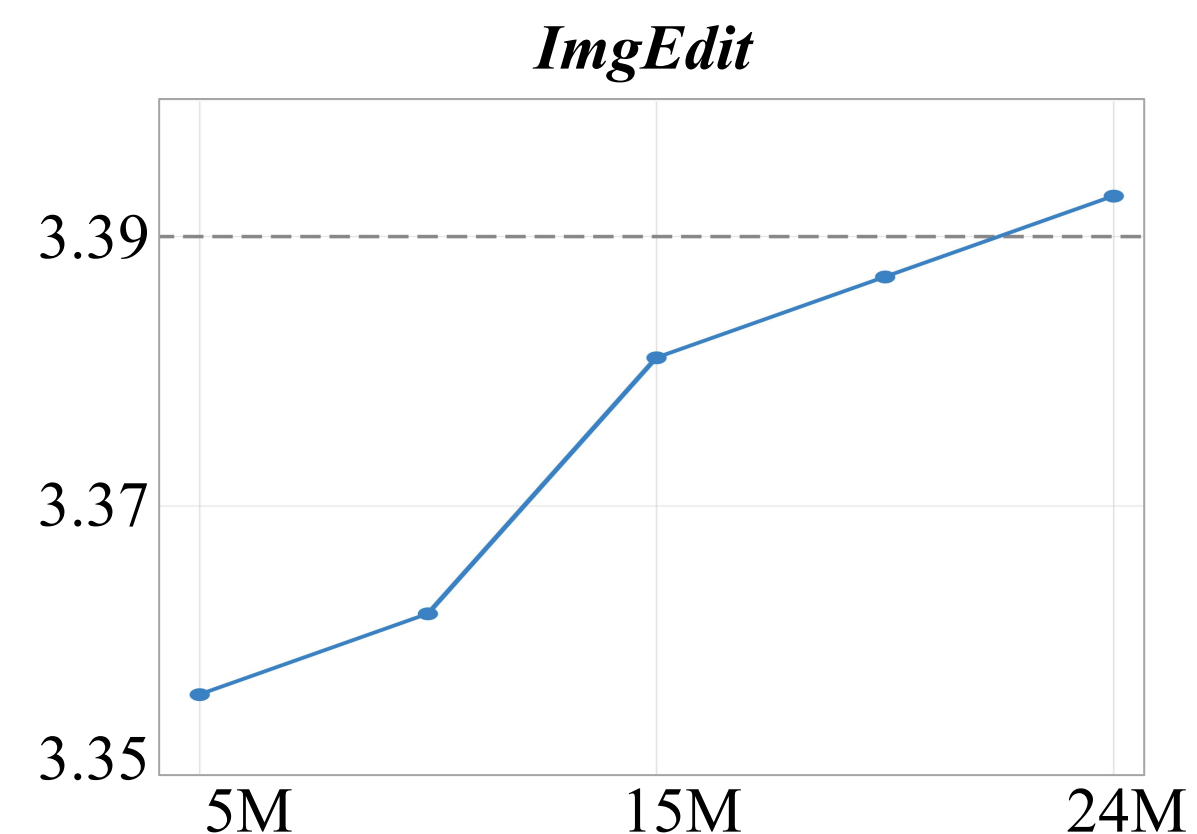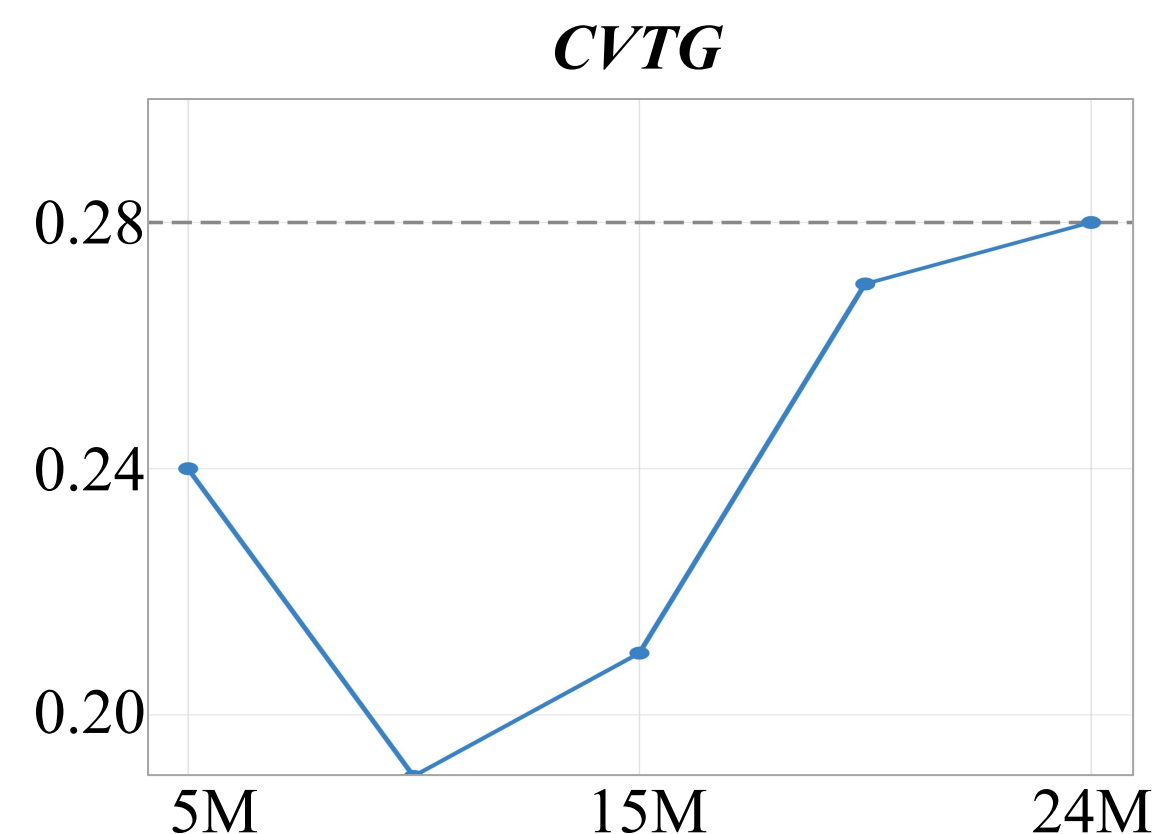

Supplement: Supplementary file 1 [file supp_data_scaling.pdf]
